# Supplementary material for: Understanding Video Transformers for Segmentation: A Survey of Application and Interpretability
Source: arXiv:2310.12296 source file (2023-10-18)
Supplement: Supplementary file 1 [file ArticleAppendix.tex]

To fully derive Kalman filtering in the linear Gaussian scenario, we follow \cite{chen2003bayesian} to clarify a few more necessary assumptions:
\begin{itemize}
  \item Noise $q$ and $r$ are \textit{Dirac delta} functions (thus zero-mean white Gaussian noise).
  \item The state and process noise are mutually independent:
  $\mathbb{E}[x_t, q_m^{T}] = 0; \mathbb{E}[x_t, r_m^{T}] = 0$, for all $n, m$.
  \item The process noise and measurement noise are mutually independent: 
  $\mathbb{E}[q_t, r_m^{T}] = 0$, for all $n, m$. 
\end{itemize}

Following the Bayesian filtering equation and the above assumptions, the mean and covariance of the likelihood $p(y_t|x_t)$ thus can be written as
\begin{equation}
\centering
    \mathbb{E}[y_t | x_t] = \mathbb{E}[H x_t + r_t] = H x_t
\label{eq:mean_likelihood}
\end{equation}
and
\begin{equation}
    Cov[y_t | x_t] = Cov[r_t] = \Sigma_{r},
\end{equation}
respectively, so the distribution of the likelihood $p(y_t|x_t)$ is considered as a Gaussian distribution in form of $\mathcal{N}(y_t - Hx_t, \Sigma_{r})$.
 
Similarly, the mean and covariance of the prior $p(x_t | y_{t-1})$ as 
\begin{equation}
    \mathbb{E}[x_t | y_{t-1}] = \mathbb{E}[F \hat{x}_{t-1} + q_t | y_{t-1}] = F \hat{x}_{t|t-1}
\label{eq:prior}
\end{equation}
and
\begin{equation}
        Cov[x_t | y_{t-1}] = Cov[x_t - \hat{x}_{t|t-1}] = Cov[e_{t|t-1}],
\end{equation}
respectively, where $\hat{x}_{t|t-1}$ is the state vector prediction at time $t$ given observations up to time $t-1$ and $e_{t|t-1}$ is the state error vector, representing the difference between the real state, $x_t$, after observing the real measurement, $y_t$, and the predicted state, $\hat{x}_{t|t-1}$. Moving forward, we denote the $Cov[e_{t|t-1}]$ as $P_{t|t-1}$, to represent the \textbf{error covariance} that the filter thinks the estimate error has. Finally, the prior distribution $p(x_t | y_{t-1})$ can be expressed as a Gaussian distribution of the form of $\mathcal{N}(x_t - \hat{x}_{t|t-1}, P_{t|t-1})$.

Assuming the measurement evidence, $p(y_t | y_{t-1})$, as an unrelated constant value, the desired posterior $p(x_t | y_t)$ under the Kalman assumption can be deduced as
\begin{equation}
\begin{aligned}
    p(x_t | y_t) &\propto \mathcal{N}(y_t - Hx_t, \Sigma_{r}) \times \mathcal{N}(x_t - \hat{x}_{t|t-1}, P_{t|t-1}) \\
    &\propto exp\left(-\frac{1}{2}(y_t - Hx_t)^{T} \Sigma_{r}^{-1} (y_t - Hx_t) -\frac{1}{2}(x_t - \hat{x}_{t|t-1})^{T} P_{t|t-1}^{-1} (x_t - \hat{x}_{t|t-1})\right).
\end{aligned}
\label{eq:kf_posterior}
\end{equation}
In this equation, the unknown and desired variable is the optimal state and we can resort to the Maximum A Posteriori (MAP) estimate to find the optimal $x^{MAP}$ such that
\begin{equation}
    \frac{\delta log(p(x_t | y_t))}{\delta x_t}|_{x_t = x^{MAP}} = 0.
\label{eq:kalman_MAP}
\end{equation}
Using this objective function on Equation \ref{eq:kf_posterior} yields
\begin{equation}
    \hat{x}_{t}^{MAP} = (H^{T} \Sigma_{r} H + P_{t|t-1}^{-1})^{-1}
                      \times (P_{t|t-1}^{-1} \hat{x}_{t|t-1} + H^T \Sigma_{r} y_t).
\label{eq:kf_deduct_1}
\end{equation}

The simplification of the above matrix can be achieved with the Woodbury matrix identity \cite{woodbury1950inverting} (also known as matrix inversion lemma), which states that
\begin{equation}
    (A + UCV)^{-1} = A^{-1} - A^{-1}U(C^{-1} + VA^{-1}U)^{-1}VA^{-1}.
\label{eq:inverse_lemma}
\end{equation}
So, Equation \ref{eq:kf_deduct_1} can be expressed as
\begin{equation}
\begin{aligned}
    \hat{x}_{t}^{MAP} &= (P_{t|t-1} - P_{t|t-1}(\Sigma_{r} + HP_{t|t-1}H^{T})^{-1}HP_{t|t-1}) \times (P_{t|t-1}^{-1} \hat{x}_{t|t-1} + H^T \Sigma_{r} y_t) \\
    &= \hat{x}_{t|t-1} - K_t H \hat{x}_{t|t-1} + (P_{t|t-1}H\Sigma_{r}^{-1} - 
    P_{t|t-1}H^{-1}(\Sigma_{r} + H P_{t|t-1} H^{T})^{-1}H P_{t|t-1} H^{T} \Sigma_{r}^{-1}) y_t \\
    &= \hat{x}_{t|t-1} - K_t H \hat{x}_{t|t-1} + K_t [(H P_{t|t-1} H^T + \Sigma_{r}) \Sigma_{r}^{-1} - H P_{t|t-1} H^T \Sigma_{r}^{-1}]y_t \\
    &= \hat{x}_{t|t-1} - K_t H \hat{x}_{t|t-1} + K_t y_t \\
    &= \hat{x}_{t|t-1} + K_t(y_t - H\hat{x}_{t|t-1}),
\end{aligned}
\end{equation}
where $K_t = P_{t|t-1}H^{T} (HP_{t|t-1}H^{T} + \Sigma{r})^{-1}$.

Since both the real state, $x_t$, and the prior estimation state, $\hat{x}_{t|t-1}$, get propagated by the transition matrix $F$ along time, so do their residuals:
\begin{equation}
    \begin{aligned}
        e_{t|t-1} &= x_{t} - \hat{x}_{t|t-1} \\
                  &= Fx_t + q_t - Fx_{t-1}^{MAP} \\
                  &= Fe_{t-1}^{MAP} + q_t
    \end{aligned}
\end{equation}
and
\begin{equation}
    \begin{aligned}
        P_{t|t-1} &= Cov[e_{t|t-1}] \\
                  &= FP_{t-1}F^{T} + \Sigma q.
    \end{aligned}
\label{eq:error_prop}
\end{equation}

Accordingly, the updated error, $e_t$, comes from the reduction of the real state, $x_t$, and the updated state, $\hat{x}_t^{MAP}$, by
\begin{equation}
    \begin{aligned}
        e_t &= x_t - \hat{x}_t^{MAP} \\
            &= x_t - \hat{x}_{t|t-1} - K_t ( y_t - H\hat{x}_{t|t-1}) \\
            &= e_{t|t-1} K_t (He_{t|t-1} + q_t) \\
            &= (I - K_t H)e_{t|t-1} - K_t q_t.
    \end{aligned}
\label{eq:error_mean}
\end{equation}
So, the updated error covariance, $P_t$, can be written as
\begin{equation}
    \begin{aligned}
    P_t &= Cov[e_t] \\
        &= (I - K_t H) P_{t|t-1} (I - K_t H )^{T} + K_t \Sigma q K_t^{T} \\
        &= (I - K_t H) P_{t|t-1},
    \end{aligned}
\label{eq:error_update}
\end{equation}
with $I$ indicating the identity matrix.
