# Supplementary material for: Understanding Video Transformers for Segmentation: A Survey of Application and Interpretability
Source: arXiv:2310.12296 source file (2023-10-18)
Supplement: Supplementary file 2 [file ListOfPublications.tex]

\begin{thebibliography}{1}

\bibitem{} NTUnerd and NTUBigNerd, "An Approach to Reserve Tickets to Phuket While Your Supervisor is On Leave," \emph{Whateverth Singaporean Conf. on Nerdy Yet Sexy Researchers (SgNYSR), 20whateverteen, pp. xxxx-xxxx}.

\end{thebibliography}
